# Supplementary material for: Hierarchical Planning for Long-Horizon Manipulation with Geometric and Symbolic Scene Graphs
Source: arXiv:2012.07277 source file (2021-03-30)
Supplement: Supplementary file 1 [file supp.tex]

\section*{Appendix}

\subsection{Environments}
Storage environments
shelf sizes?

Digital twin in simulation.

\subsection{Real Robot Setup}
Franka Emika Robot
3-4 images at each region at fixed locations

Moveit with RRT. 

\subsection{Neural Network Model}
preimage netwowrk

reachability network

Adam optimizer
Learning rate 1e-4, with reduced plateau scheduler
Pytorch
